# Supplementary material for: Separating the Material and Geometry Contribution to the Circular Dichroism of Chiral Objects Made from Chiral Media
Source: arXiv:2401.06664 source file (2024-01-12)
Supplement: Supplementary file 1 [file SeparatingCD_SI.pdf]

# Supplemental Material

—

## Separating the Material and Geometry Contribution to the Circular Dichroism of Chiral Objects Made from Chiral Media

Lukas Rebholz,<sup>1,\*</sup> Marjan Krstić,<sup>1</sup> Benedikt Zerulla,<sup>2</sup> Mateusz Pawlak,<sup>3</sup>  
Wiktor Lewandowski,<sup>3</sup> Ivan Fernandez-Corbaton,<sup>2</sup> and Carsten Rockstuhl<sup>1,2</sup>

<sup>1</sup>*Institute of Theoretical Solid State Physics,*

*Karlsruhe Institute of Technology, Karlsruhe, Germany*

<sup>2</sup>*Institute of Nanotechnology, Karlsruhe Institute of Technology, Karlsruhe, Germany*

<sup>3</sup>*Faculty of Chemistry, University of Warsaw, Warsaw, Poland*

(Dated: January 11, 2024)

---

\* lukas.rebholz@kit.edu

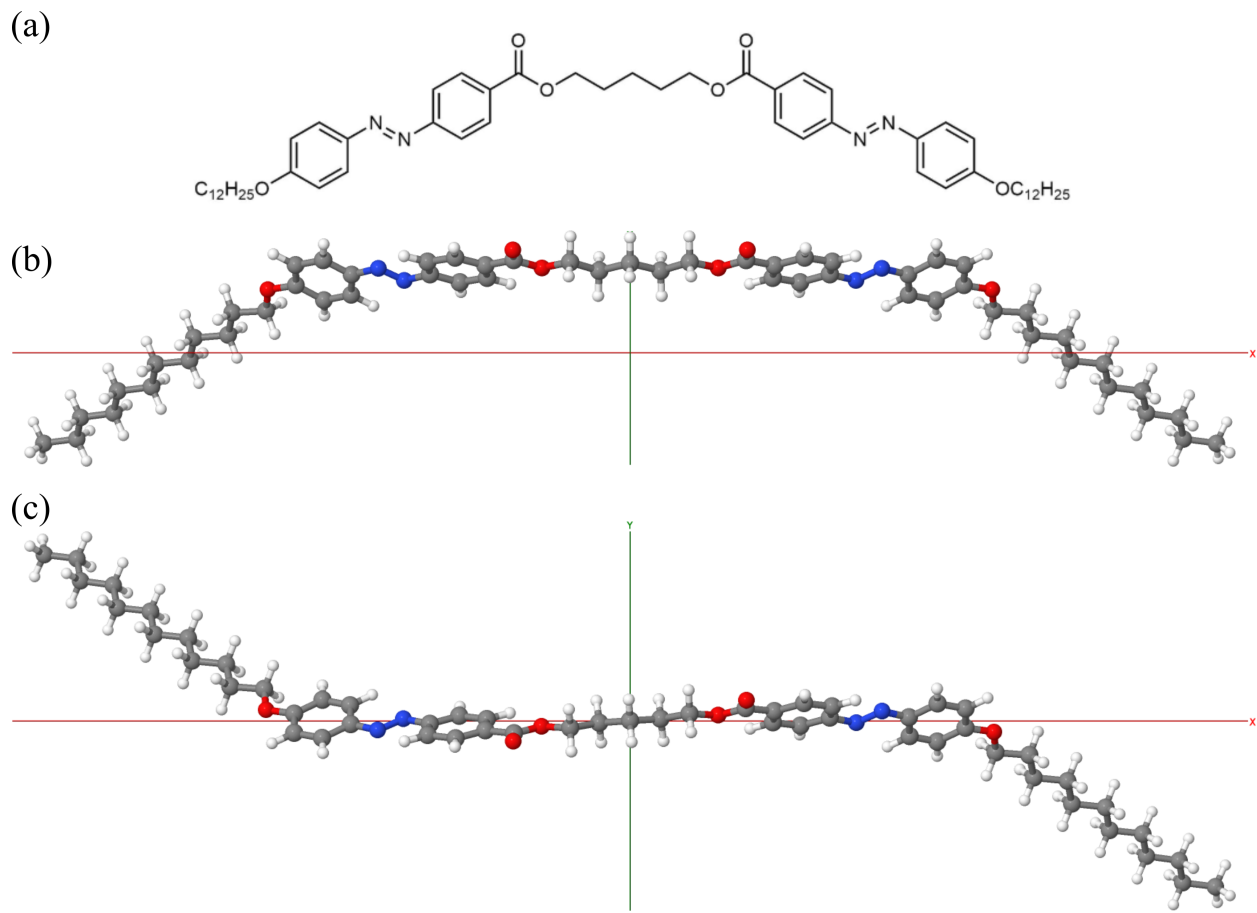

Fig. S1. (a) Chemical 2D representation of the molecular structure of the 12OAzO5AzO12 molecule. Adapted from [1]. (b) Top-down view along the  $-z$  axis of the DFT optimized structure of the achiral conformer of the 12OAzO5AzO12 molecule. (c) Top-down view of the DFT optimized structure of the 12OAzO5AzO12 molecule, having chiral structure and optical properties. Structures from (b) and (c) are energetically degenerate, but all further studies reported in the manuscript were performed on the chiral structure shown in (c).

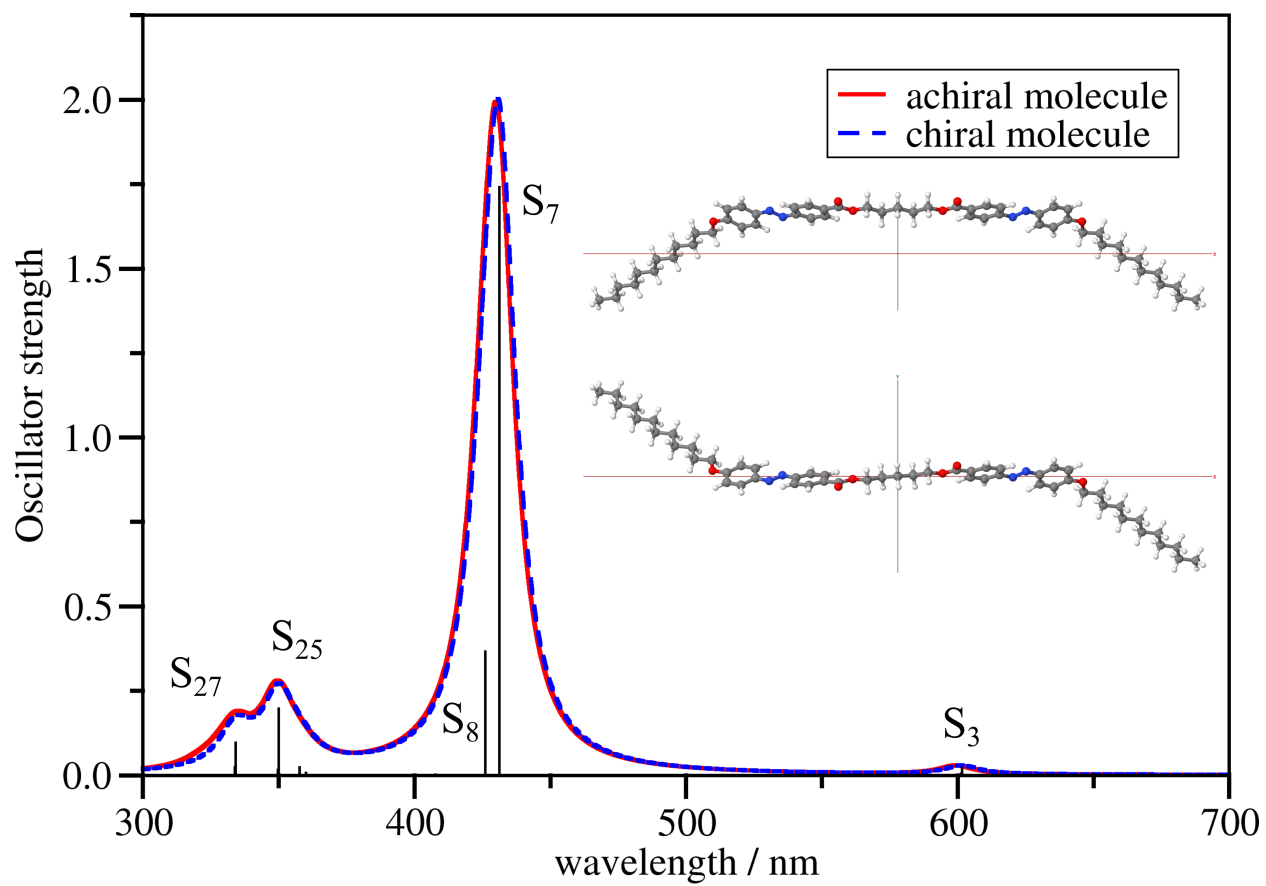

Fig. S2. UV-Vis absorption spectrum of both the achiral and chiral molecules of 12OAzo5AzoO12. Black vertical lines represent oscillator strengths of the electronic transitions of the chiral conformer. Lorentzian line-shape with 15 nm at full-width at half-maximum was used to convolute the spectra.

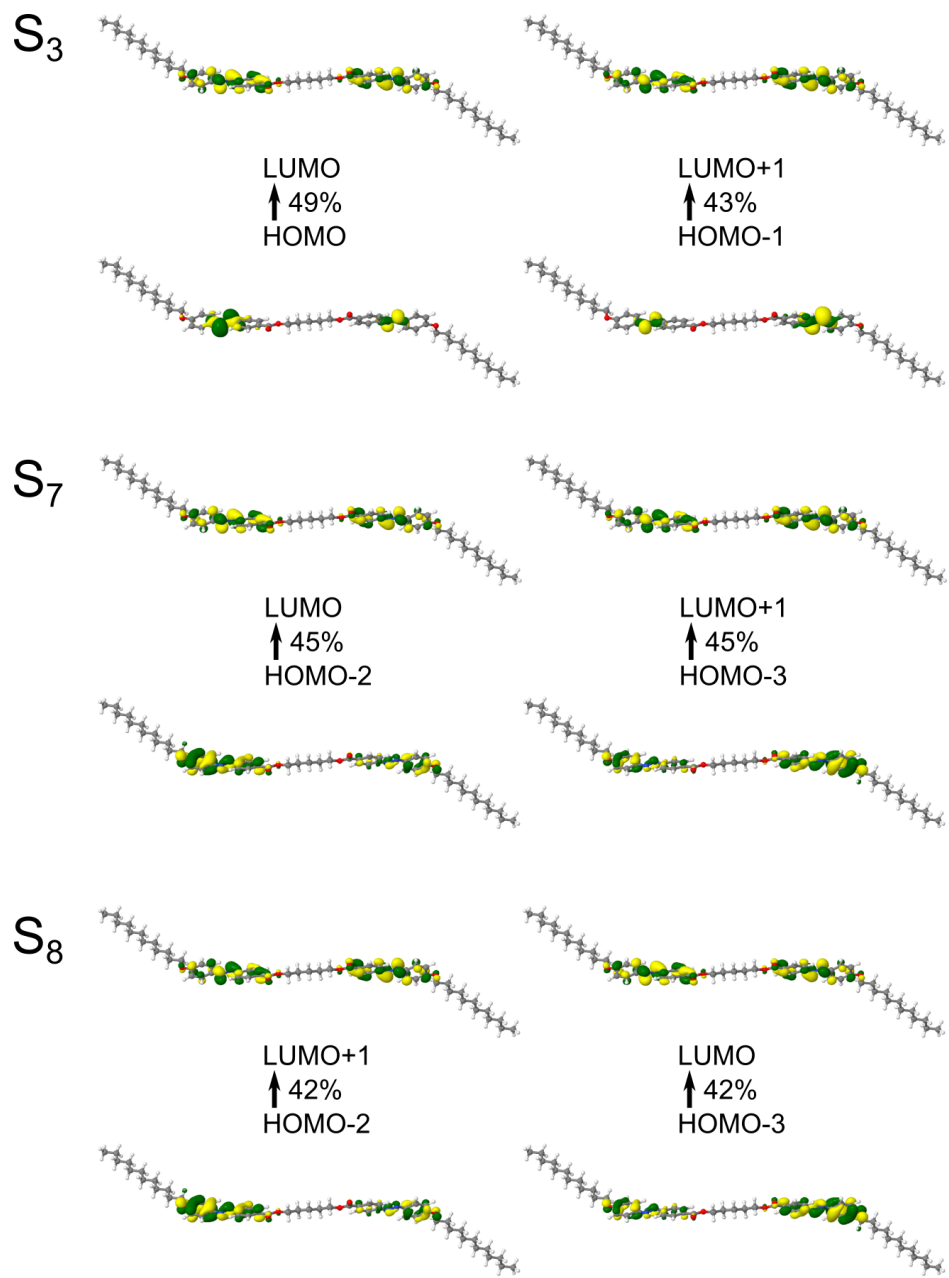

Fig. S3. Analysis of leading molecular orbital contributions to the discrete singlet electronic transitions  $S_3$ ,  $S_7$  and  $S_8$  of the chiral 12OAzO5AzoO12 molecule from the Figure S2. Green and yellow surfaces correspond to the positive and negative part of the molecular orbital for the isosurface of values  $\pm 0.03$ .

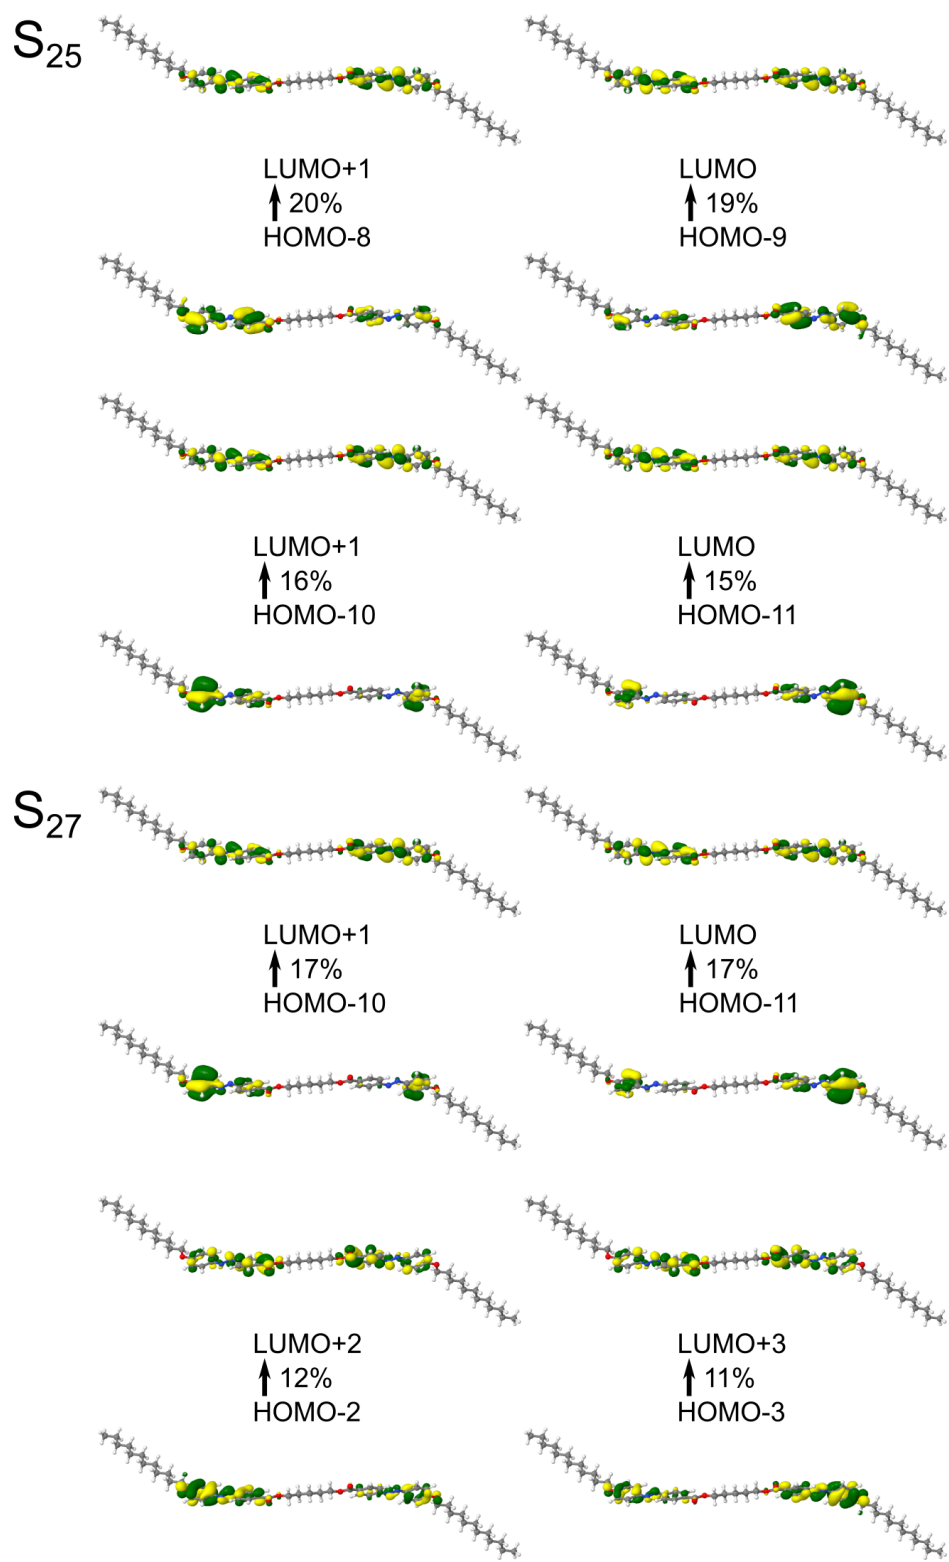

Fig. S4. Analysis of leading molecular orbital contributions to the discrete singlet electronic transitions  $S_5$  and  $S_{27}$  of the chiral 12OAzO5AzO12 molecule from the Figure S2. Green and yellow surfaces correspond to the positive and negative part of the molecular orbital for the isosurface of values  $\pm 0.03$ .

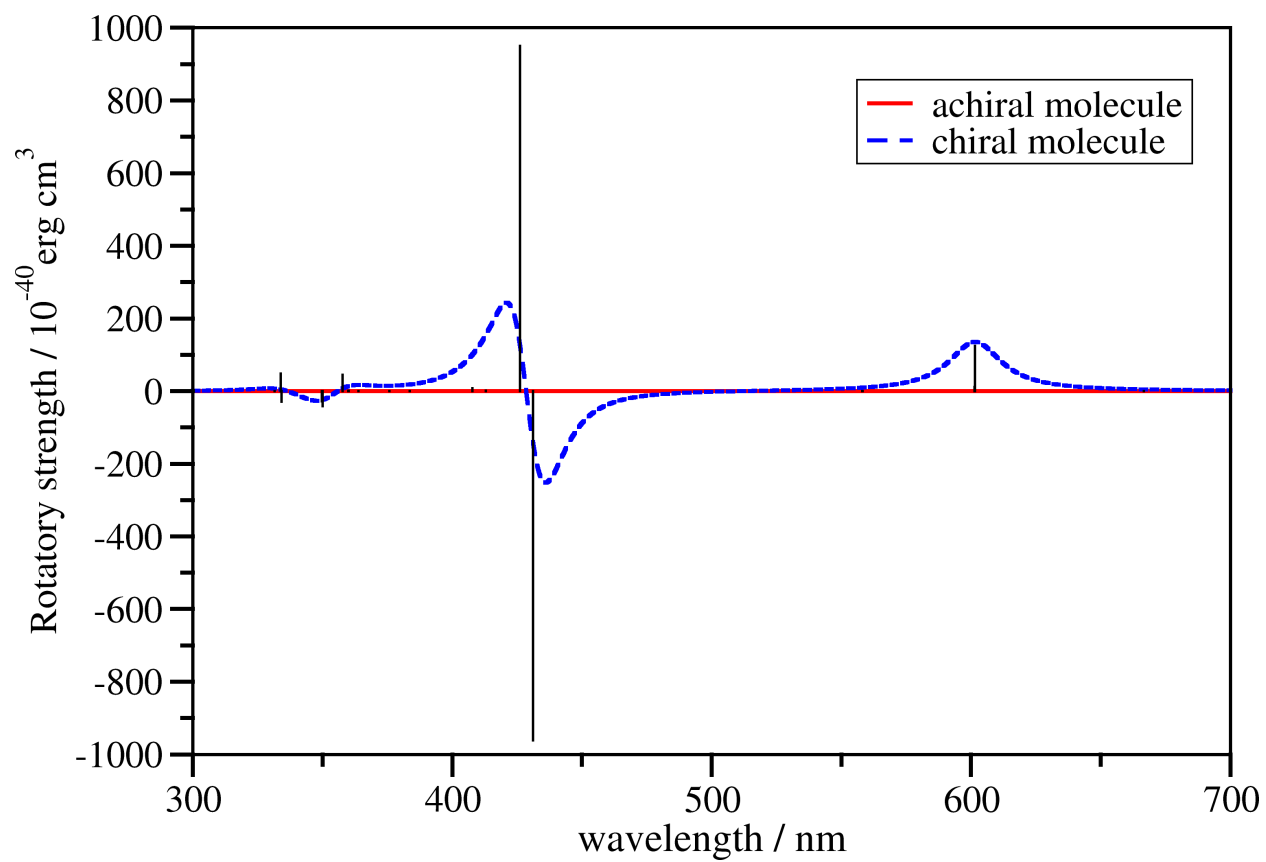

Fig. S5. Discrete rotatory strengths and convoluted spectrum of the chiral 12OAzo5AzoO12 molecule using Lorentzian line-shape with 25 nm at full-width at half-maximum. The achiral conformer of the 12OAzo5AzoO12 molecule does not show any circular dichroism signal (solid red line).

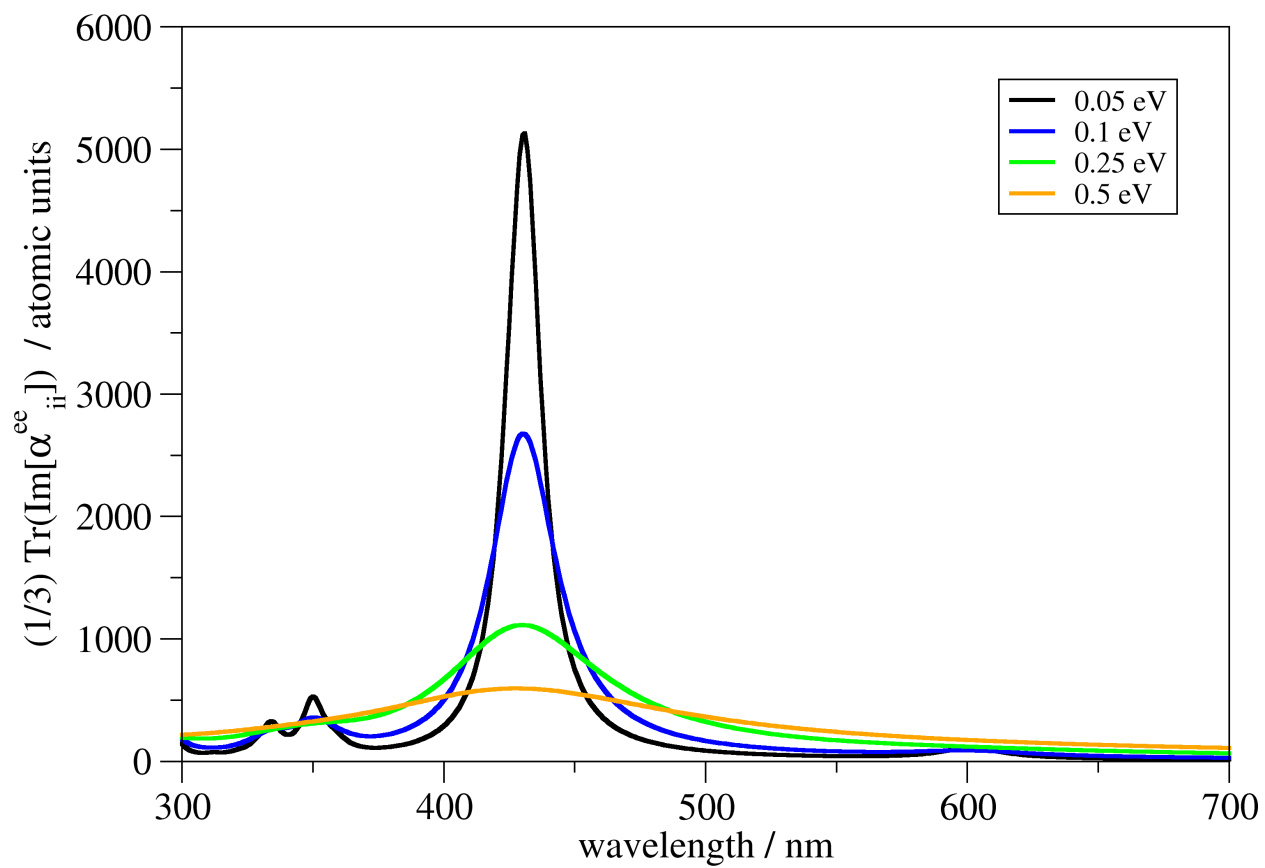

Fig. S6. The influence of the selected empirical damping on the values of the electric-electric dynamic polarizabilities and overall absorption spectrum constructed from those polarizabilities for chiral 12OAzO5AzoO12 molecule.

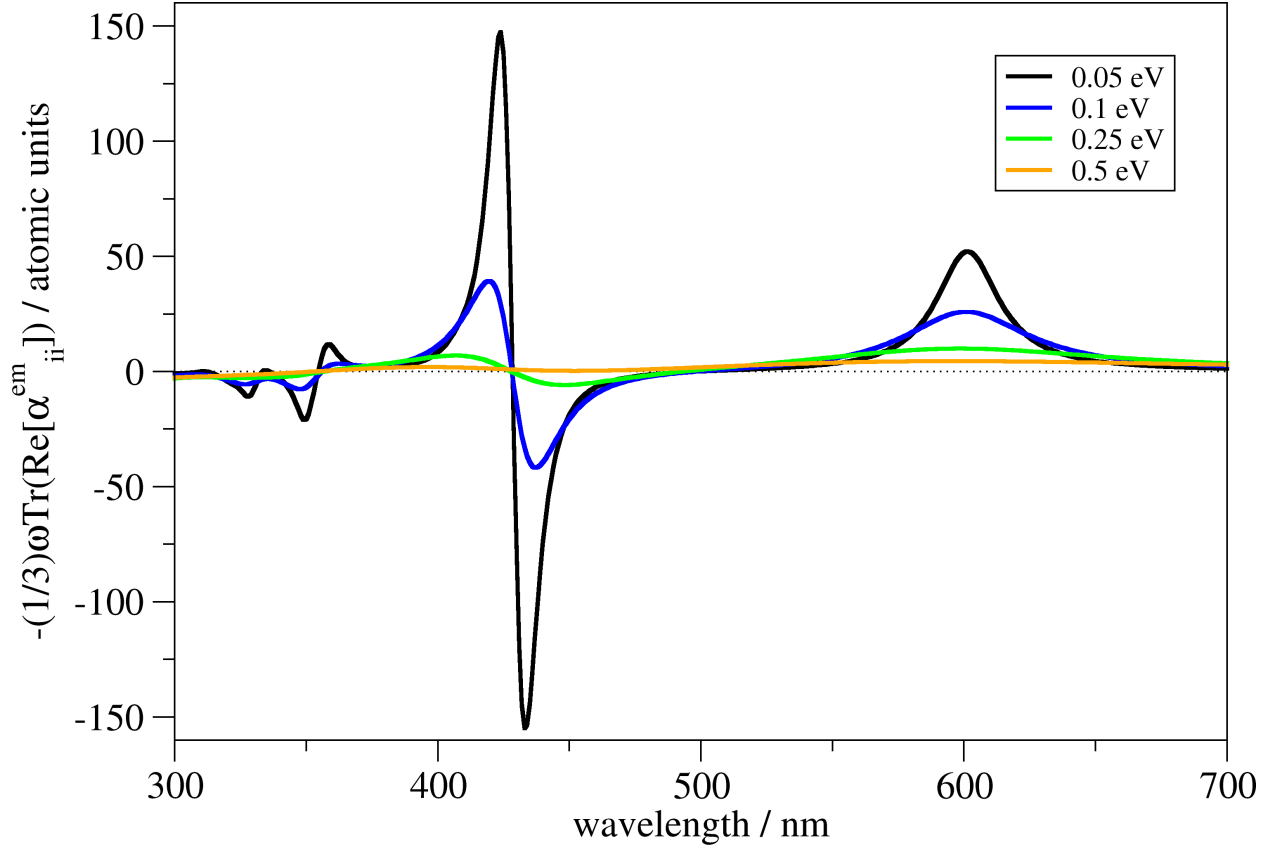

Fig. S7. The influence of the selected empirical damping on the values of the electric-magnetic dynamic polarizabilities and overall CD spectrum constructed from those polarizabilities for chiral 12OAzo5AzoO12 molecule.

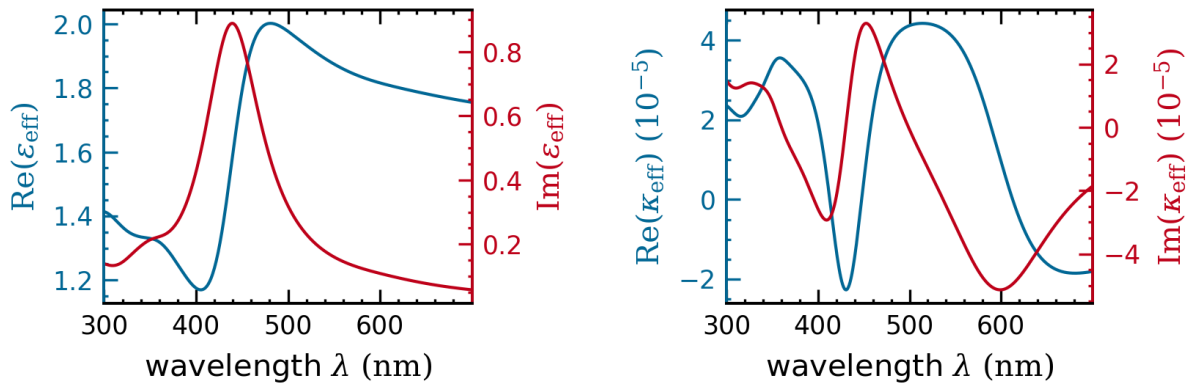

Fig. S8. Effective relative permittivity  $\epsilon_{\text{eff}}$  (left) and effective material chirality  $\kappa_{\text{eff}}$  (right) used in the study of non-resonant helices. The material parameters are computed for the chiral configuration of 12OAzo5AzoO12 (see Fig. S1(c)) assuming a molecular concentration of  $c = 3 \times 10^{26} \text{ m}^{-3}$ .

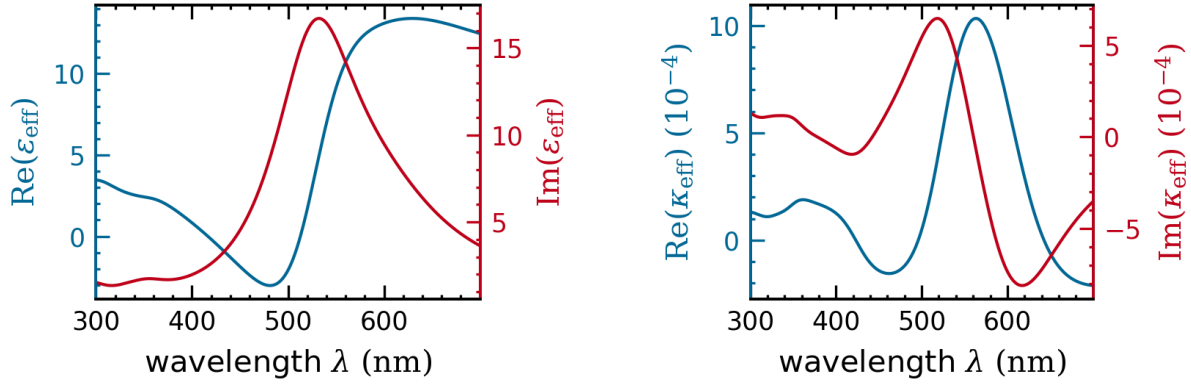

Fig. S9. Effective relative permittivity  $\epsilon_{\text{eff}}$  (left) and effective material chirality  $\kappa_{\text{eff}}$  (right) used in the study of resonant tetrahedral arrangements of spheres. The material parameters are computed for the chiral configuration of 12OAzO5AzoO12 (see Fig. S1(c)) assuming a molecular concentration of  $c = 1.2 \times 10^{27} \text{ m}^{-3}$ .

- 
- [1] A. Jedrych, M. Pawlak, E. Gorecka, W. Lewandowski, and M. M. Wojcik, Light-responsive supramolecular nanotubes-based chiral plasmonic assemblies, *ACS Nano* **17**, 5548 (2023).
